# Supplementary material for: PrefillOnly: An Inference Engine for Prefill-only Workloads in Large Language Model Applications
Source: arXiv:2505.07203 source file (2025-05-12)
Supplement: Supplementary file 1 [file appendix.tex]

% \section{Estimating the storage overhead of \name}
% \label{appendix:storage-overhead}

% We take the technical specification of DOVEs constellation to estimate this overhead.
% We first estimate the space required for storing captured images.
% Let the area that the satellite can download during one ground contact be $a$ km$^2$.
% The storage space required to store this $a$ km$^2$ imagery is thus $0.87a$ MB, where the coefficient 0.87 is the megabytes required to encode 1km$^2$ area, estimated by the fact that each image captured by Doves constellation is 300 MB, with a resolution of 6600$\times$4400 and a ground sampling distance of 3 $m$.
% Thus, the storage space used to store captured imagery is approximately $2 \times 0.87a$ MB, where this 2$\times$ factor is because the ground keeps the captured imagery for two consecutive ground contacts to make sure the downloading is successful~\cite{leoconn}.
% \name stores the reference images of all locations that each satellite will download, totaling at most $160a$ km$^2$, since the satellite revisits the same location once every 10-15 days~\cite{sentinel-2-revisit} and the maximum amount of ground contact it can have is 240 times, assuming that the satellite can have ground contact during every 90-minute orbit.
% Since \name's downsampling technique compresses the reference images by $2601\times$. As a result, the total storage space for reference images is at most $0.08a MB$, 9\% of the space for storing captured imagery.
